# Supplementary material for: Constant Size Molecular Descriptors For Use With Machine Learning
Source: arXiv:1701.06649 ancillary file (2017-01-23)
Supplement: Supplementary file 1 [file supplemental.pdf]

# Supporting information for: Constant Size Molecular Descriptors For Use With Machine Learning

Christopher R. Collins,† Geoffrey J. Gordon,‡ O. Anatole von Lilienfeld,¶ and David J. Yaron*,†

†*Department of Chemistry, Carnegie Mellon University, Pittsburgh, Pennsylvania 15213 United States*

‡*Machine Learning Department, Carnegie Mellon University, Pittsburgh, Pennsylvania 15213 United States*

¶*Department of Chemistry, Institute of Physical Chemistry and National Center for Computational Design and Discovery of Novel Materials (MARVEL), University of Basel, 4056 Basel, Switzerland*

## 1 Bond lengths for connectivity counts

The connectivity count features in Section 5.3 of the main manuscript rely on identifying either the presence of a bond or the bond order. The values in Table S1 were summed to give the atom separation corresponding to the upper limit of a given bond type. The bond order is assigned based on this upper limit and the maximum allowed bond order between the respective elements. For features that rely on only the presence of a bond, a bond is assumes to be present if the atoms are closer than the cutoff for a single bond.

Table S1: All distances listed are in Å.

| Element | Single | Aromatic | Double | Triple |
|---|---|---|---|---|
| C | 0.850 | 0.720 | 0.690 | 0.620 |
| Cl | 1.045 | | | |
| F | 1.230 | | | |
| H | 0.600 | | | |
| N | 0.740 | 0.655 | 0.630 | 0.565 |
| O | 0.695 | 0.620 | 0.590 | 0.530 |
| P | 1.110 | 0.985 | 0.945 | |
| S | 1.070 | 0.945 | 0.905 | |

# 2 Implementation of encoded distance features

For the encoding distance features of Section 5.4 of the main manuscript, there are a few parameters that must be adjusted. These include the $\beta$ for the encoding functions of Table 2, the start and end points of the grids, and the number of grid points. These parameters were chosen based on model performance for QM7 atomization energies, along with the time and memory involved in the computations. The chosen values are $\beta = 20$, and a grid with $N_{grid}$ = 100 points between 0.2Å and 6Å. The following shows how model performance varies with each parameter in turn, holding the remaining parameters at their chosen value.

Figure S1 shows that there is a broad range of values for $\beta$ that give roughly equal performance on QM7 atomization energies. We chose 20 for $\beta$ because it is in the center of this range. For large $\beta$, the encoding function approaches that of the spike encoding function, leading to poor performance. The dependence on $\beta$ for $\mathbf{2^{LP}}$ is similar to that seen for $\mathbf{2^{NP}}$ in Figure S1, so $\beta = 20$ was used for both normal and logistic encoding functions.

Figures S2 and S3 show model performance and computation time as a function of the number of grid points, $N_{grid}$. The computation time increases nearly linearly with $N_{grid}$. The model performance improves substantially up to about $N_{grid} = 50$ and then levels off. A value of 100 was chosen as a reasonable compromise between performance and computation time.

The dependence of model performance on the start and end points of the grid are shown

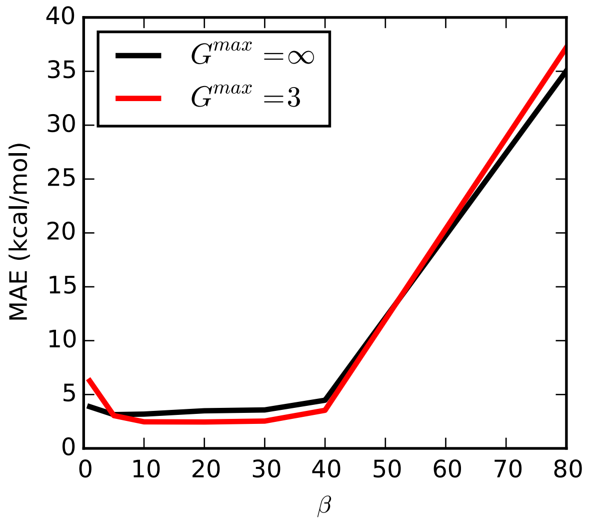


Figure S1: Dependence of MAE on $\beta$ for KRR models of the QM7 atomization energy. The models use $\mathbf{2^{NP}}$ as a feature vector.

in Figures S5 and S6, respectively. The results are consistent with the distribution of atomic separations in Figure S4. For $G^{max}$ of 3, the distributions lie between 0.8 and 4 Å. For $G^{max} = \infty$, the distributions lie between 0.8 and about 6 Å. The model performance is independent of starting point for values below about 1.0 Å (Figure S5). As the end point is increased in Figure S6, performance initially improves, until about 6 Å and then degrades for larger values. This degradation can be attributed to the loss of grid resolution in the main range of values. We chose a start value of 0.2Å and an end value of 6.0 Å to span the distribution of atomic separations in the QM7 data set, while retaining good model performance.

To reduce computation, we elected to remove all encoded ranges where there were no examples (in the case of the QM7 data set, this means 14 encoded ranges).

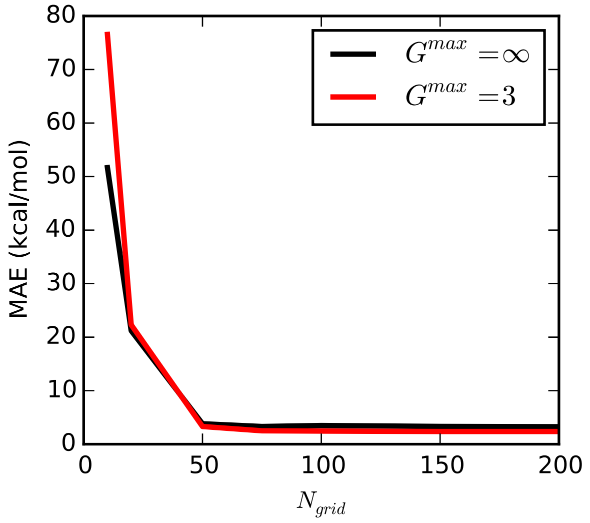


Figure S2: Dependence of MAE on number of grid points for KRR models of the QM7 atomization energy. The models use $\mathbf{2^{NP}}$ as a feature vector.

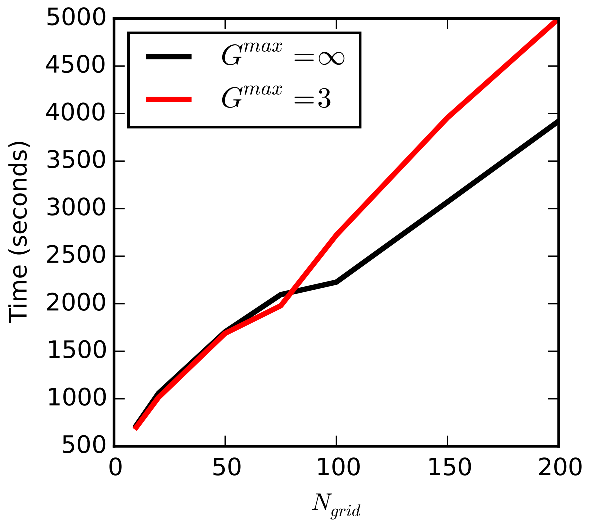


Figure S3: The relation between the time required for training/testing and the number of grid points.

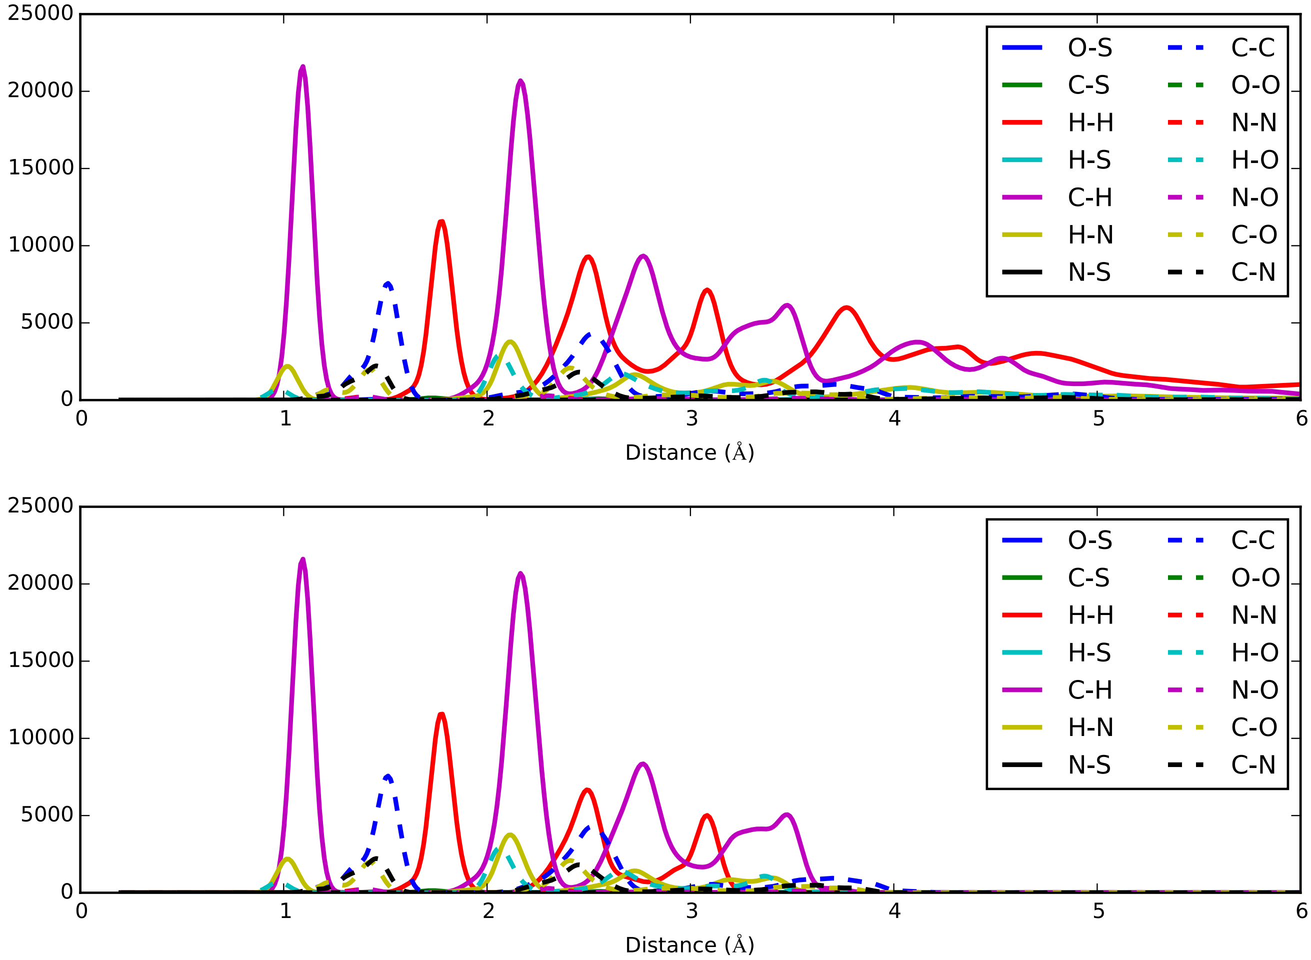


Figure S4: Distribution of bond distances in the QM7 data set, using the normal probability distribution as the encoding function. The upper panel has no restriction on atomic separations. The lower panel is for $G^{max} = 3$.

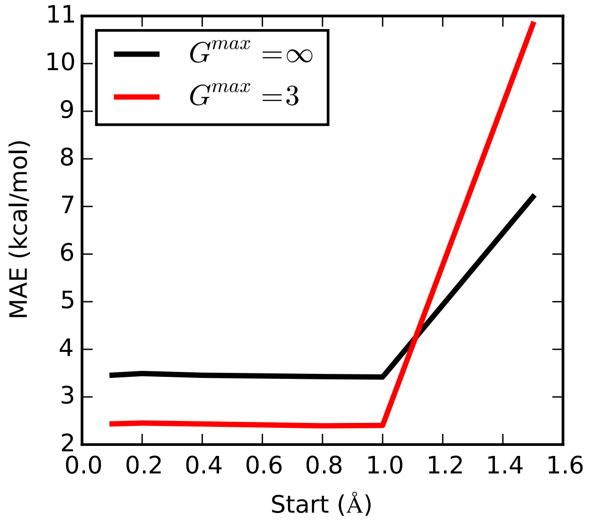


Figure S5: Dependence of MAE on the starting point for grid for KRR models of the QM7 atomization energy. The models use $\mathbf{2}^{\boldsymbol{NP}}$ as a feature vector.

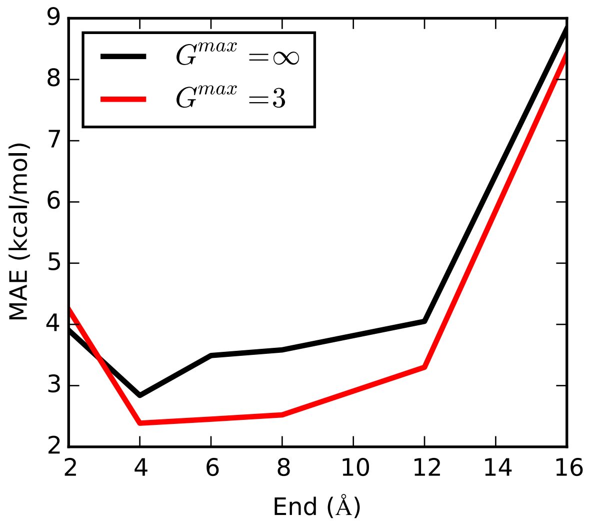


Figure S6: Dependence of MAE on the ending point for grid for KRR models of the QM7 atomization energy. The models use $\mathbf{2}^{\boldsymbol{NP}}$ as a feature vector.

# 3 Results

Table S2: For the results dealing with learning rates (Table 5, Figure 4, and Figure 5), the following sets of hyperparameters were used.

| Feature | $\alpha$ | $\gamma$ | Kernel |
|---|---|---|---|
| $\mathbf{12^{NP}3^{B}4^{B}}$ | 1e-7 | 1e-5 | gauss |
| BoB | 1e-9 | 1e-5 | laplace |
| $\mathbf{2^{LC}}$ | 1e-9 | 1e-5 | gauss |
| $\mathbf{2^{B}}$ | 1e-7 | 0.001 | gauss |

Tables S3 and S4 list MAEs from LRR and KRR models, respectively, of QM7 atomization energies. Fold lists the standard deviation across the 5 folds. Unless otherwise specified, all encoded distance features use the default values of the previous section. The notation for feature vectors is as in the main manuscript, with the addition of subscripts to encoded distance features to indicate parameters that differ from their default values. Integer subscripts refer to the value of $G^{max}$, with no subscript indicating $G^{max} = \infty$ . Other changes from default values are listed as {key: value}, pairs.

| Name | LRR | Fold | $\alpha$ |
|---|---|---|---|
| 1 | 15.7007 | 0.2515 | 0.001 |
| 1 $2^B$ | 8.5378 | 0.1485 | 0.1 |
| 1 $2^B$ 3 | 6.2088 | 0.1291 | 0.1 |
| 1 $2^B$ 3 4 | 5.2756 | 0.1588 | 0.1 |
| 1 $2^B$ 3 4 5 | 4.2939 | 0.1087 | 1.0 |
| 1 $2^B$ 3 $4^B$ | 4.5085 | 0.0763 | 1.0 |
| 1 $2^B$ 3 $4^B$ 5 | 3.7927 | 0.1324 | 1.0 |
| 1 $2^B$ $3^B$ | 5.6513 | 0.1438 | 0.01 |
| 1 $2^B$ $3^B$ 4 | 4.9384 | 0.1694 | 0.1 |
| 1 $2^B$ $3^B$ 4 5 | 4.0619 | 0.1123 | 1.0 |
| 1 $2^B$ $3^B$ $4^B$ | 4.4827 | 0.0792 | 1.0 |
| 1 $2^B$ $3^B$ $4^B$ 5 | 3.7473 | 0.1413 | 1.0 |

| | | | |
|---|---|---|---|
| 1 $2^{LC}$ | 2.8034 | 0.1242 | 0.01 |
| 1 $2^{LC}$ 3 | 2.5502 | 0.0735 | 0.01 |
| 1 $2^{LC}$ 3 4 | 2.4542 | 0.0660 | 0.01 |
| 1 $2^{LC}$ 3 $4^{B}$ | 2.0353 | 0.0332 | 0.1 |
| 1 $2^{LC}$ $3^{B}$ | 2.2607 | 0.0374 | 0.01 |
| 1 $2^{LC}$ $3^{B}$ 4 | 2.2352 | 0.0436 | 0.01 |
| 1 $2^{LC}$ $3^{B}$ $4^{B}$ | 2.0144 | 0.0394 | 0.1 |
| 1 $2_1^{LC}$ | 6.3336 | 0.1485 | 0.01 |
| 1 $2_1^{LC}$ 3 | 5.1905 | 0.1364 | 0.01 |
| 1 $2_1^{LC}$ 3 4 | 4.3768 | 0.4273 | 0.001 |
| 1 $2_1^{LC}$ 3 $4^{B}$ | 3.6673 | 0.1029 | 1.0 |
| 1 $2_1^{LC}$ $3^{B}$ | 4.5679 | 0.2295 | 0.001 |
| 1 $2_1^{LC}$ $3^{B}$ 4 | 3.9977 | 0.1484 | 0.01 |
| 1 $2_1^{LC}$ $3^{B}$ $4^{B}$ | 3.6471 | 0.1256 | 1.0 |
| 1 $2_2^{LC}$ | 2.8404 | 0.0561 | 0.001 |
| 1 $2_2^{LC}$ 3 | 2.7304 | 0.1345 | 0.001 |
| 1 $2_2^{LC}$ 3 4 | 2.5988 | 0.0486 | 0.01 |
| 1 $2_2^{LC}$ 3 $4^{B}$ | 2.0242 | 0.0405 | 0.1 |
| 1 $2_2^{LC}$ $3^{B}$ | 2.4390 | 0.0456 | 0.01 |
| 1 $2_2^{LC}$ $3^{B}$ 4 | 2.3134 | 0.0534 | 0.01 |
| 1 $2_2^{LC}$ $3^{B}$ $4^{B}$ | 2.0186 | 0.0464 | 0.1 |
| 1 $2_3^{LC}$ | 2.5950 | 0.0745 | 0.01 |
| 1 $2_3^{LC}$ 3 | 2.4634 | 0.0660 | 0.01 |
| 1 $2_3^{LC}$ 3 4 | 2.3820 | 0.0663 | 0.01 |
| 1 $2_3^{LC}$ 3 4 5 | 2.3616 | 0.0714 | 0.1 |
| 1 $2_3^{LC}$ 3 $4^{B}$ | 1.8184 | 0.0555 | 0.1 |
| 1 $2_3^{LC}$ 3 $4^{B}$ 5 | 1.8551 | 0.0652 | 0.1 |

| | | | |
|---|---|---|---|
| 1 $2_3^{LC}$ $3^B$ | 2.1421 | 0.0584 | 0.01 |
| 1 $2_3^{LC}$ $3^B$ 4 | 2.1157 | 0.0730 | 0.01 |
| 1 $2_3^{LC}$ $3^B$ 4 5 | 2.1545 | 0.0914 | 0.1 |
| 1 $2_3^{LC}$ $3^B$ $4^B$ | 1.8220 | 0.0763 | 0.1 |
| 1 $2_3^{LC}$ $3^B$ $4^B$ 5 | 1.8467 | 0.0761 | 0.1 |
| 1 $2_3^{LC}$ {'$\beta$': 30.0} | 2.4833 | 0.0662 | 0.01 |
| 1 $2_3^{LC}$ {'$\beta$': 30.0} $3^B$ | 2.0831 | 0.0481 | 0.01 |
| 1 $2_3^{LC}$ {'$\beta$': 30.0} $3^B$ $4^B$ | 1.7737 | 0.0677 | 0.1 |
| 1 $2_3^{NC}$ | 2.4833 | 0.0574 | 0.01 |
| 1 $2_3^{NC}$ $3^B$ | 2.0900 | 0.0476 | 0.01 |
| 1 $2_3^{NC}$ $3^B$ $4^B$ | 1.7791 | 0.0677 | 0.1 |
| 1 $2_3^{NC}$ {'$\beta$': 30.0} | 2.4728 | 0.0823 | 0.1 |
| 1 $2_3^{NC}$ {'$\beta$': 30.0} $3^B$ | 2.0745 | 0.0614 | 0.1 |
| 1 $2_3^{NC}$ {'$\beta$': 30.0} $3^B$ $4^B$ | 1.7480 | 0.0625 | 0.1 |
| 1 $2_3^{NP}$ | 2.4711 | 0.0775 | 0.01 |
| 1 $2_3^{NP}$ $3^B$ | 2.0992 | 0.0402 | 0.01 |
| 1 $2_3^{NP}$ $3^B$ $4^B$ | 1.7641 | 0.0353 | 0.1 |
| 1 $2_3^{SC}$ | 2.8994 | 0.0542 | 0.1 |
| 1 $2_3^{SC}$ $3^B$ | 2.4362 | 0.0608 | 0.1 |
| 1 $2_3^{SC}$ $3^B$ $4^B$ | 2.0145 | 0.0427 | 1.0 |
| 1 $2_3^{SC}$ {'$\beta$': 30.0} | 2.8994 | 0.0542 | 0.1 |
| 1 $2_3^{SC}$ {'$\beta$': 30.0} $3^B$ | 2.4362 | 0.0608 | 0.1 |
| 1 $2_3^{SC}$ {'$\beta$': 30.0} $3^B$ $4^B$ | 2.0145 | 0.0427 | 1.0 |
| 1 $2_4^{LC}$ | 2.9074 | 0.1089 | 0.01 |
| 1 $2_4^{LC}$ 3 | 2.5179 | 0.1151 | 0.001 |
| 1 $2_4^{LC}$ 3 4 | 2.4741 | 0.1138 | 0.001 |
| 1 $2_4^{LC}$ 3 $4^B$ | 2.0616 | 0.0287 | 0.1 |

| | | | |
|---|---|---|---|
| 1 $2_4^{LC}$ $3^B$ | 2.2613 | 0.0317 | 0.01 |
| 1 $2_4^{LC}$ $3^B$ 4 | 2.2239 | 0.0428 | 0.01 |
| 1 $2_4^{LC}$ $3^B$ $4^B$ | 2.0277 | 0.0417 | 0.1 |
| 1 $2_5^{LC}$ | 2.8299 | 0.1217 | 0.01 |
| 1 $2_5^{LC}$ 3 | 2.5707 | 0.0637 | 0.01 |
| 1 $2_5^{LC}$ 3 4 | 2.4725 | 0.0653 | 0.01 |
| 1 $2_5^{LC}$ 3 $4^B$ | 2.0565 | 0.0341 | 0.1 |
| 1 $2_5^{LC}$ $3^B$ | 2.2785 | 0.0364 | 0.01 |
| 1 $2_5^{LC}$ $3^B$ 4 | 2.2473 | 0.0509 | 0.01 |
| 1 $2_5^{LC}$ $3^B$ $4^B$ | 2.0376 | 0.0422 | 0.1 |
| 1 $2_6^{LC}$ | 2.8041 | 0.1241 | 0.01 |
| 1 $2_6^{LC}$ 3 | 2.5481 | 0.0700 | 0.01 |
| 1 $2_6^{LC}$ 3 4 | 2.4512 | 0.0637 | 0.01 |
| 1 $2_6^{LC}$ 3 $4^B$ | 2.0369 | 0.0359 | 0.1 |
| 1 $2_6^{LC}$ $3^B$ | 2.2585 | 0.0379 | 0.01 |
| 1 $2_6^{LC}$ $3^B$ 4 | 2.2323 | 0.0444 | 0.01 |
| 1 $2_6^{LC}$ $3^B$ $4^B$ | 2.0161 | 0.0419 | 0.1 |
| 1 $2_7^{LC}$ | 2.8045 | 0.1230 | 0.01 |
| 1 $2_7^{LC}$ 3 | 2.5507 | 0.0724 | 0.01 |
| 1 $2_7^{LC}$ 3 4 | 2.4539 | 0.0650 | 0.01 |
| 1 $2_7^{LC}$ 3 $4^B$ | 2.0343 | 0.0342 | 0.1 |
| 1 $2_7^{LC}$ $3^B$ | 2.2605 | 0.0363 | 0.01 |
| 1 $2_7^{LC}$ $3^B$ 4 | 2.2346 | 0.0434 | 0.01 |
| 1 $2_7^{LC}$ $3^B$ $4^B$ | 2.0136 | 0.0404 | 0.1 |
| 1 Bag of Bonds | 9.7804 | 0.1511 | 1.0 |
| 1 Bag of Bonds 3 | 6.2550 | 0.1560 | 0.1 |
| 1 Bag of Bonds 3 4 | 5.9116 | 0.1627 | 1.0 |

| | | | |
|---|---|---|---|
| 1 Bag of Bonds 3 $4^B$ | 4.1550 | 0.1231 | 1.0 |
| 1 Bag of Bonds $3^B$ | 4.6733 | 0.1413 | 1.0 |
| 1 Bag of Bonds $3^B$ 4 | 4.5066 | 0.1433 | 1.0 |
| 1 Bag of Bonds $3^B$ $4^B$ | 4.0767 | 0.1245 | 1.0 |
| $1^C$ | 11.2675 | 0.2300 | 0.001 |
| $1^C$ $2^B$ | 8.5248 | 0.1427 | 0.01 |
| $1^C$ $2^B$ 3 | 6.2042 | 0.1376 | 0.1 |
| $1^C$ $2^B$ 3 4 | 5.2733 | 0.1665 | 0.1 |
| $1^C$ $2^B$ 3 4 5 | 4.3145 | 0.1368 | 1.0 |
| $1^C$ $2^B$ 3 $4^B$ | 4.4981 | 0.0840 | 1.0 |
| $1^C$ $2^B$ 3 $4^B$ 5 | 3.8035 | 0.1505 | 1.0 |
| $1^C$ $2^B$ $3^B$ | 5.6428 | 0.1452 | 0.1 |
| $1^C$ $2^B$ $3^B$ 4 | 4.9329 | 0.1640 | 0.1 |
| $1^C$ $2^B$ $3^B$ 4 5 | 4.0597 | 0.1125 | 0.1 |
| $1^C$ $2^B$ $3^B$ $4^B$ | 4.5067 | 0.0847 | 1.0 |
| $1^C$ $2^B$ $3^B$ $4^B$ 5 | 3.8092 | 0.1528 | 1.0 |
| $1^C$ $2^{LC}$ | 2.7767 | 0.1252 | 0.01 |
| $1^C$ $2^{LC}$ 3 | 2.5489 | 0.0551 | 0.01 |
| $1^C$ $2^{LC}$ 3 4 | 2.4661 | 0.0452 | 0.01 |
| $1^C$ $2^{LC}$ 3 $4^B$ | 2.0435 | 0.0318 | 0.1 |
| $1^C$ $2^{LC}$ $3^B$ | 2.2727 | 0.0429 | 0.01 |
| $1^C$ $2^{LC}$ $3^B$ 4 | 2.2458 | 0.0423 | 0.01 |
| $1^C$ $2^{LC}$ $3^B$ $4^B$ | 2.0221 | 0.0351 | 0.1 |
| $1^C$ $2_1^{LC}$ | 6.2415 | 0.1723 | 0.01 |
| $1^C$ $2_1^{LC}$ 3 | 5.1853 | 0.1395 | 0.01 |
| $1^C$ $2_1^{LC}$ 3 4 | 4.3757 | 0.4312 | 0.001 |
| $1^C$ $2_1^{LC}$ 3 $4^B$ | 3.6495 | 0.0919 | 1.0 |

| | | | |
|---|---|---|---|
| $1^{C}\ 2_{1}^{LC}\ 3^{B}$ | 4.5926 | 0.2839 | 0.001 |
| $1^{C}\ 2_{1}^{LC}\ 3^{B}\ 4$ | 3.9817 | 0.1503 | 0.01 |
| $1^{C}\ 2_{1}^{LC}\ 3^{B}\ 4^{B}$ | 3.6316 | 0.1142 | 1.0 |
| $1^{C}\ 2_{2}^{LC}$ | 2.8002 | 0.1120 | 0.001 |
| $1^{C}\ 2_{2}^{LC}\ 3$ | 2.7532 | 0.1308 | 0.001 |
| $1^{C}\ 2_{2}^{LC}\ 3\ 4$ | 2.6000 | 0.0489 | 0.01 |
| $1^{C}\ 2_{2}^{LC}\ 3\ 4^{B}$ | 2.0303 | 0.0342 | 0.1 |
| $1^{C}\ 2_{2}^{LC}\ 3^{B}$ | 2.4398 | 0.0451 | 0.01 |
| $1^{C}\ 2_{2}^{LC}\ 3^{B}\ 4$ | 2.3183 | 0.0530 | 0.01 |
| $1^{C}\ 2_{2}^{LC}\ 3^{B}\ 4^{B}$ | 2.0154 | 0.0384 | 0.1 |
| $1^{C}\ 2_{3}^{LC}$ | 2.5549 | 0.0811 | 0.01 |
| $1^{C}\ 2_{3}^{LC}\ 3$ | 2.4589 | 0.0631 | 0.01 |
| $1^{C}\ 2_{3}^{LC}\ 3\ 4$ | 2.3737 | 0.0684 | 0.01 |
| $1^{C}\ 2_{3}^{LC}\ 3\ 4^{B}$ | 1.8185 | 0.0554 | 0.1 |
| $1^{C}\ 2_{3}^{LC}\ 3^{B}$ | 2.1548 | 0.0589 | 0.01 |
| $1^{C}\ 2_{3}^{LC}\ 3^{B}\ 4$ | 2.1209 | 0.0784 | 0.01 |
| $1^{C}\ 2_{3}^{LC}\ 3^{B}\ 4^{B}$ | 1.8163 | 0.0693 | 0.1 |
| $1^{C}\ 2_{3}^{LC}\ 3\ 4\ 5$ | 2.3945 | 0.0598 | 0.1 |
| $1^{C}\ 2_{3}^{LC}\ 3\ 4^{B}\ 5$ | 1.8658 | 0.0673 | 0.1 |
| $1^{C}\ 2_{3}^{LC}\ 3^{B}\ 4\ 5$ | 2.1644 | 0.0843 | 0.1 |
| $1^{C}\ 2_{3}^{LC}\ 3^{B}\ 4^{B}\ 5$ | 1.8469 | 0.0785 | 0.1 |
| $1^{C}\ 2_{4}^{LC}$ | 2.8441 | 0.2314 | 0.001 |
| $1^{C}\ 2_{4}^{LC}\ 3$ | 2.5473 | 0.1145 | 0.001 |
| $1^{C}\ 2_{4}^{LC}\ 3\ 4$ | 2.4922 | 0.0605 | 0.01 |
| $1^{C}\ 2_{4}^{LC}\ 3\ 4^{B}$ | 2.0597 | 0.0330 | 0.1 |
| $1^{C}\ 2_{4}^{LC}\ 3^{B}$ | 2.2617 | 0.0366 | 0.01 |
| $1^{C}\ 2_{4}^{LC}\ 3^{B}\ 4$ | 2.2218 | 0.0388 | 0.01 |

| | | | |
|---|---|---|---|
| $1^C\ 2_4^{LC}\ 3^B\ 4^B$ | 2.0374 | 0.0430 | 0.1 |
| $1^C\ 2_5^{LC}$ | 2.8058 | 0.1242 | 0.01 |
| $1^C\ 2_5^{LC}\ 3$ | 2.5593 | 0.1398 | 0.001 |
| $1^C\ 2_5^{LC}\ 3\ 4$ | 2.4842 | 0.0536 | 0.01 |
| $1^C\ 2_5^{LC}\ 3\ 4^B$ | 2.0639 | 0.0341 | 0.1 |
| $1^C\ 2_5^{LC}\ 3^B$ | 2.2910 | 0.0404 | 0.01 |
| $1^C\ 2_5^{LC}\ 3^B\ 4$ | 2.2564 | 0.0473 | 0.01 |
| $1^C\ 2_5^{LC}\ 3^B\ 4^B$ | 2.0444 | 0.0399 | 0.1 |
| $1^C\ 2_6^{LC}$ | 2.7776 | 0.1262 | 0.01 |
| $1^C\ 2_6^{LC}\ 3$ | 2.5467 | 0.0530 | 0.01 |
| $1^C\ 2_6^{LC}\ 3\ 4$ | 2.4624 | 0.0444 | 0.01 |
| $1^C\ 2_6^{LC}\ 3\ 4^B$ | 2.0454 | 0.0340 | 0.1 |
| $1^C\ 2_6^{LC}\ 3^B$ | 2.2706 | 0.0433 | 0.01 |
| $1^C\ 2_6^{LC}\ 3^B\ 4$ | 2.2429 | 0.0429 | 0.01 |
| $1^C\ 2_6^{LC}\ 3^B\ 4^B$ | 2.0239 | 0.0376 | 0.1 |
| $1^C\ 2_7^{LC}$ | 2.7775 | 0.1240 | 0.01 |
| $1^C\ 2_7^{LC}\ 3$ | 2.5489 | 0.0541 | 0.01 |
| $1^C\ 2_7^{LC}\ 3\ 4$ | 2.4657 | 0.0441 | 0.01 |
| $1^C\ 2_7^{LC}\ 3\ 4^B$ | 2.0429 | 0.0327 | 0.1 |
| $1^C\ 2_7^{LC}\ 3^B$ | 2.2727 | 0.0415 | 0.01 |
| $1^C\ 2_7^{LC}\ 3^B\ 4$ | 2.2453 | 0.0416 | 0.01 |
| $1^C\ 2_7^{LC}\ 3^B\ 4^B$ | 2.0214 | 0.0361 | 0.1 |
| $1^C$ Bag of Bonds | 7.8937 | 0.1697 | 0.1 |
| $1^C$ Bag of Bonds 3 | 5.4190 | 0.1682 | 1.0 |
| $1^C$ Bag of Bonds 3 4 | 5.1525 | 0.1559 | 1.0 |
| $1^C$ Bag of Bonds 3 $4^B$ | 4.1234 | 0.1261 | 1.0 |
| $1^C$ Bag of Bonds $3^B$ | 4.5804 | 0.1591 | 1.0 |

| | | | |
|---|---|---|---|
| $1^C$ Bag of Bonds $3^B$ 4 | 4.4246 | 0.1461 | 1.0 |
| $1^C$ Bag of Bonds $3^B$ $4^B$ | 4.0642 | 0.1229 | 1.0 |
| 2 | 42.5581 | 0.3532 | 1.0 |
| $2^B$ | 12.916 | 0.2919 | 0.001 |
| $2^{LP}$ | 4.9019 | 0.0818 | 0.01 |
| $2^{NC}$ | 4.9497 | 0.0720 | 0.1 |
| $2^{NP}$ | 4.9553 | 0.0972 | 0.1 |
| $2^{NP}$ {'end': 12.0} | 5.8791 | 0.1431 | 0.1 |
| $2^{NP}$ {'end': 16.0} | 12.6072 | 0.2010 | 0.01 |
| $2^{NP}$ {'end': 2.0} | 6.7371 | 0.1762 | 0.001 |
| $2^{NP}$ {'end': 4.0} | 4.9788 | 0.0994 | 0.01 |
| $2^{NP}$ {'end': 6.0} | 4.9553 | 0.0972 | 0.1 |
| $2^{NP}$ {'end': 8.0} | 4.8223 | 0.0962 | 0.1 |
| $2^{NP}$ {'segments': 10} | 60.0313 | 0.9907 | 0.001 |
| $2^{NP}$ {'segments': 150} | 4.9064 | 0.0941 | 0.1 |
| $2^{NP}$ {'segments': 200} | 4.9032 | 0.0943 | 0.1 |
| $2^{NP}$ {'segments': 25} | 28.8464 | 0.4007 | 0.001 |
| $2^{NP}$ {'segments': 50} | 5.9702 | 0.0741 | 0.01 |
| $2^{NP}$ {'segments': 75} | 5.0141 | 0.1073 | 0.01 |
| $2^{NP}$ {'$\beta$': 1.0} | 6.6683 | 0.0815 | 0.001 |
| $2^{NP}$ {'$\beta$': 10.0} | 5.0004 | 0.0623 | 0.01 |
| $2^{NP}$ {'$\beta$': 2.5} | 5.8535 | 0.1770 | 0.001 |
| $2^{NP}$ {'$\beta$': 30.0} | 5.0820 | 0.1035 | 0.01 |
| $2^{NP}$ {'$\beta$': 40.0} | 6.1273 | 0.0896 | 0.01 |
| $2^{NP}$ {'$\beta$': 5.0} | 5.4152 | 0.2241 | 0.001 |
| $2^{NP}$ {'$\beta$': 80.0} | 39.5902 | 1.0179 | 1.0 |
| $2^{NP}$ {'start': 0.1} | 4.9468 | 0.0996 | 0.1 |

| | | | |
|---|---|---|---|
| $2^{NP}$ {'start': 0.2} | 4.9553 | 0.0972 | 0.1 |
| $2^{NP}$ {'start': 0.4} | 4.9298 | 0.1011 | 0.1 |
| $2^{NP}$ {'start': 0.8} | 4.9413 | 0.1028 | 0.1 |
| $2^{NP}$ {'start': 1.0} | 4.9672 | 0.0872 | 0.1 |
| $2^{NP}$ {'start': 1.5} | 11.1556 | 0.2164 | 0.1 |
| $2^{SC}$ | 6.0140 | 0.1786 | 1.0 |
| $2^{SP}$ | 132.1945 | 3.0651 | 1.0 |
| $2_1$ | 9.0548 | 0.2739 | 0.01 |
| $2_1^{LP}$ | 8.6599 | 0.4742 | 0.001 |
| $2_1^{NC}$ | 8.6347 | 0.6150 | 0.01 |
| $2_1^{NP}$ | 8.0929 | 0.2361 | 0.0001 |
| $2_1^{SC}$ | 11.2133 | 0.1713 | 1e-05 |
| $2_1^{SP}$ | 168.3545 | 1.3873 | 0.01 |
| $2_2$ | 5.2149 | 0.1719 | 0.001 |
| $2_2^{LP}$ | 5.0587 | 0.2155 | 0.0001 |
| $2_2^{NC}$ | 5.0651 | 0.0696 | 0.01 |
| $2_2^{NP}$ | 5.0130 | 0.0427 | 0.001 |
| $2_2^{SC}$ | 6.8146 | 0.1797 | 0.1 |
| $2_2^{SP}$ | 162.2208 | 1.4962 | 1.0 |
| $2_3$ | 4.5538 | 0.0915 | 0.01 |
| $2_3^{LC}$ | 4.5538 | 0.0915 | 0.01 |
| $2_3^{LC}$ {'$\beta$': 30.0} | 4.4312 | 0.0792 | 0.01 |
| $2_3^{LP}$ | 4.5203 | 0.0905 | 0.001 |
| $2_3^{NC}$ | 4.4493 | 0.0769 | 0.01 |
| $2_3^{NC}$ $2_3^{NP}$ | 4.4139 | 0.0935 | 0.01 |
| $2_3^{NC}$ {'$\beta$': 30.0} | 4.3749 | 0.1100 | 0.01 |
| $2_3^{NP}$ | 2.4711 | 0.0775 | 0.01 |

| | | | |
|---|---|---|---|
| $2_3^{NP}$ {'end': 12.0} | 5.6734 | 0.1611 | 0.001 |
| $2_3^{NP}$ {'end': 16.0} | 14.2262 | 0.3014 | 0.001 |
| $2_3^{NP}$ {'end': 4.0} | 4.3218 | 0.1182 | 0.001 |
| $2_3^{NP}$ {'end': 6.0} | 4.5121 | 0.1077 | 0.01 |
| $2_3^{NP}$ {'end': 8.0} | 4.5460 | 0.1004 | 0.01 |
| $2_3^{NP}$ {'segments': 10} | 84.1753 | 1.0094 | 0.001 |
| $2_3^{NP}$ {'segments': 150} | 4.3073 | 0.1170 | 0.001 |
| $2_3^{NP}$ {'segments': 200} | 4.3546 | 0.1049 | 0.01 |
| $2_3^{NP}$ {'segments': 25} | 33.4157 | 0.8663 | 0.001 |
| $2_3^{NP}$ {'segments': 50} | 5.6196 | 0.1571 | 0.001 |
| $2_3^{NP}$ {'segments': 75} | 4.5435 | 0.1103 | 0.01 |
| $2_3^{NP}$ {'$\beta$': 1.0} | 10.9222 | 0.3285 | 0.001 |
| $2_3^{NP}$ {'$\beta$': 10.0} | 4.6449 | 0.1176 | 0.001 |
| $2_3^{NP}$ {'$\beta$': 2.5} | 6.6183 | 0.1584 | 0.001 |
| $2_3^{NP}$ {'$\beta$': 30.0} | 4.5288 | 0.1102 | 0.01 |
| $2_3^{NP}$ {'$\beta$': 40.0} | 5.9969 | 0.0569 | 0.01 |
| $2_3^{NP}$ {'$\beta$': 5.0} | 5.5599 | 0.2342 | 0.001 |
| $2_3^{NP}$ {'$\beta$': 80.0} | 46.6440 | 0.8325 | 0.001 |
| $2_3^{NP}$ {'start': 0.1} | 4.4750 | 0.1120 | 0.01 |
| $2_3^{NP}$ {'start': 0.2} | 4.5121 | 0.1077 | 0.01 |
| $2_3^{NP}$ {'start': 0.4} | 4.4493 | 0.1035 | 0.01 |
| $2_3^{NP}$ {'start': 0.8} | 4.3680 | 0.1384 | 0.001 |
| $2_3^{NP}$ {'start': 1.0} | 4.3581 | 0.1290 | 0.001 |
| $2_3^{NP}$ {'start': 1.5} | 20.8561 | 0.3221 | 0.01 |
| $2_3^{SC}$ | 5.7663 | 0.1090 | 1.0 |
| $2_3^{SC}$ {'$\beta$': 30.0} | 5.7663 | 0.1090 | 1.0 |
| $2_3^{SP}$ | 147.6294 | 2.7820 | 1.0 |

| | | | |
|---|---|---|---|
| $2_4$ | 5.1088 | 0.0731 | 0.01 |
| $2_4^{LP}$ | 5.0595 | 0.1353 | 0.001 |
| $2_4^{NC}$ | 4.9912 | 0.0933 | 0.01 |
| $2_4^{NP}$ | 5.0452 | 0.1022 | 0.01 |
| $2_4^{SC}$ | 6.5754 | 0.1611 | 1.0 |
| $2_4^{SP}$ | 141.6751 | 3.1076 | 1.0 |
| $2_5$ | 5.2917 | 0.1083 | 0.01 |
| $2_5^{LP}$ | 5.2350 | 0.1373 | 0.01 |
| $2_5^{NC}$ | 5.2325 | 0.1401 | 0.01 |
| $2_5^{NP}$ | 5.2367 | 0.1354 | 0.01 |
| $2_5^{SC}$ | 6.8206 | 0.2061 | 1.0 |
| $2_5^{SP}$ | 136.9339 | 3.3614 | 1.0 |
| $2_6$ | 5.2651 | 0.1060 | 0.01 |
| $2_6^{LP}$ | 5.2299 | 0.1349 | 0.01 |
| $2_6^{NC}$ | 5.2170 | 0.1565 | 0.01 |
| $2_6^{NP}$ | 5.2317 | 0.1632 | 0.01 |
| $2_6^{SC}$ | 6.8510 | 0.1936 | 1.0 |
| $2_6^{SP}$ | 134.5053 | 2.7396 | 1.0 |
| $2_7$ | 5.2689 | 0.1012 | 0.01 |
| $2_7^{LP}$ | 5.2327 | 0.1306 | 0.01 |
| $2_7^{NC}$ | 5.2210 | 0.1516 | 0.01 |
| $2_7^{NP}$ | 5.2346 | 0.1578 | 0.01 |
| $2_7^{SC}$ | 6.8454 | 0.1966 | 1.0 |
| $2_7^{SP}$ | 134.0674 | 2.7591 | 1.0 |
| 3 | 58.6948 | 0.7411 | 1.0 |
| $3^B$ | 9.0619 | 0.3880 | 0.01 |
| 4 | 94.2483 | 1.1164 | 1.0 |

| | | | |
|---|---|---|---|
| $4^B$ | 81.5092 | 0.6791 | 1.0 |
| 5 | 102.1410 | 1.6964 | 10.0 |
| $5^B$ | 102.4255 | 1.5005 | 1.0 |
| Bag of Bonds | 9.7960 | 0.1587 | 0.01 |
| Bag of Bonds {'strip atoms': True} | 17.3518 | 0.2901 | 0.01 |
| Bag of Bonds$_1$ | 12.0466 | 0.2862 | 0.01 |
| Bag of Bonds$_1$ {'strip atoms': True} | 33.0308 | 0.2570 | 1.0 |
| Bag of Bonds$_2$ | 9.1210 | 0.2327 | 0.01 |
| Bag of Bonds$_2$ {'strip atoms': True} | 38.0673 | 0.7031 | 0.1 |
| Bag of Bonds$_3$ | 10.1130 | 0.2195 | 0.01 |
| Bag of Bonds$_3$ {'strip atoms': True} | 34.5855 | 0.6927 | 1.0 |
| Bag of Bonds$_4$ | 10.0033 | 0.1903 | 0.01 |
| Bag of Bonds$_4$ {'strip atoms': True} | 27.7330 | 0.5014 | 1.0 |
| Bag of Bonds$_5$ | 9.8274 | 0.2079 | 0.01 |
| Bag of Bonds$_5$ {'strip atoms': True} | 23.7519 | 0.2201 | 0.1 |
| Bag of Bonds$_6$ | 9.7265 | 0.1909 | 0.01 |
| Bag of Bonds$_6$ {'strip atoms': True} | 21.4671 | 0.2877 | 0.01 |
| Bag of Bonds$_7$ | 9.7240 | 0.1696 | 0.01 |
| Bag of Bonds$_7$ {'strip atoms': True} | 20.8799 | 0.2830 | 0.01 |
| Coulomb Matrix | 27.0624 | 0.4680 | 0.01 |
| Coulomb Matrix$_1$ | 29.4228 | 0.5601 | 0.001 |
| Coulomb Matrix$_2$ | 29.2594 | 0.3798 | 0.01 |
| Coulomb Matrix$_3$ | 30.8664 | 0.2111 | 0.1 |
| Coulomb Matrix$_4$ | 29.5230 | 0.2349 | 0.1 |
| Coulomb Matrix$_5$ | 29.0555 | 0.4645 | 0.01 |
| Coulomb Matrix$_6$ | 29.0772 | 0.5091 | 0.01 |
| Coulomb Matrix$_7$ | 29.1617 | 0.5299 | 0.01 |

| | | | |
|---|---|---|---|
| Null | 179.0180 | 0.0771 | 0.001 |

Table S3: LRR Results

In the following table, the kernel options are for the Gaussian Kernel (gauss) and the Laplacian Kernel (laplace). The hyperparameters $\alpha$ and $\gamma$ correspond to the regularization term, and the parameter of the kernel respectively.

| Name | KRR | Fold | $\alpha$ | $\gamma$ | Kernel |
|---|---|---|---|---|---|
| 1 | 14.5830 | 0.2586 | 1e-07 | 1e-03 | gauss |
| 1 $2^B$ | 6.8788 | 0.0190 | 1e-05 | 1e-03 | gauss |
| 1 $2^B$ 3 | 5.2761 | 0.1257 | 1e-11 | 1e-07 | gauss |
| 1 $2^B$ 3 4 | 3.6420 | 0.1186 | 1e-11 | 1e-07 | laplace |
| 1 $2^B$ 3 4 5 | 3.9640 | 0.1660 | 1e-07 | 1e-07 | gauss |
| 1 $2^B$ 3 $4^B$ | 4.1313 | 0.1067 | 1e-09 | 1e-07 | gauss |
| 1 $2^B$ 3 $4^B$ 5 | 3.3964 | 0.1324 | 1e-07 | 1e-07 | gauss |
| 1 $2^B$ $3^B$ | 4.5148 | 0.1139 | 1e-11 | 1e-07 | laplace |
| 1 $2^B$ $3^B$ 4 | 3.4005 | 0.0678 | 1e-11 | 1e-07 | laplace |
| 1 $2^B$ $3^B$ 4 5 | 3.4207 | 0.2662 | 1e-09 | 1e-07 | gauss |
| 1 $2^B$ $3^B$ $4^B$ | 3.8680 | 0.1343 | 1e-11 | 1e-07 | laplace |
| 1 $2^B$ $3^B$ $4^B$ 5 | 3.3731 | 0.1299 | 1e-07 | 1e-07 | gauss |
| 1 $2^{LC}$ | 2.1640 | 0.0583 | 1e-09 | 1e-07 | gauss |
| 1 $2^{LC}$ 3 | 2.0375 | 0.0674 | 1e-09 | 1e-07 | gauss |
| 1 $2^{LC}$ 3 4 | 1.9351 | 0.0283 | 1e-09 | 1e-07 | gauss |
| 1 $2^{LC}$ 3 $4^B$ | 1.7372 | 0.0394 | 1e-09 | 1e-07 | gauss |
| 1 $2^{LC}$ $3^B$ | 1.8000 | 0.0338 | 1e-09 | 1e-07 | gauss |
| 1 $2^{LC}$ $3^B$ 4 | 1.7596 | 0.0264 | 1e-09 | 1e-07 | gauss |
| 1 $2^{LC}$ $3^B$ $4^B$ | 1.7155 | 0.0340 | 1e-09 | 1e-07 | gauss |
| 1 $2_1^{LC}$ | 5.1025 | 0.0572 | 1e-07 | 1e-07 | laplace |

| | | | | | |
|---|---|---|---|---|---|
| 1 $2_1^{LC}$ 3 | 4.4376 | 0.0748 | 1e-07 | 1e-07 | laplace |
| 1 $2_1^{LC}$ 3 4 | 3.6197 | 0.0916 | 1e-09 | 1e-07 | gauss |
| 1 $2_1^{LC}$ 3 $4^B$ | 3.2523 | 0.1262 | 1e-07 | 1e-07 | laplace |
| 1 $2_1^{LC}$ $3^B$ | 3.9978 | 0.0997 | 1e-09 | 1e-07 | gauss |
| 1 $2_1^{LC}$ $3^B$ 4 | 3.3872 | 0.1052 | 1e-09 | 1e-07 | gauss |
| 1 $2_1^{LC}$ $3^B$ $4^B$ | 3.2175 | 0.0902 | 1e-07 | 1e-07 | laplace |
| 1 $2_2^{LC}$ | 1.8764 | 0.0790 | 1e-11 | 1e-07 | gauss |
| 1 $2_2^{LC}$ 3 | 1.8268 | 0.0397 | 1e-11 | 1e-07 | gauss |
| 1 $2_2^{LC}$ 3 4 | 1.7407 | 0.0265 | 1e-11 | 1e-07 | gauss |
| 1 $2_2^{LC}$ 3 $4^B$ | 1.6869 | 0.0118 | 1e-09 | 1e-07 | gauss |
| 1 $2_2^{LC}$ $3^B$ | 1.7257 | 0.0711 | 1e-11 | 1e-07 | gauss |
| 1 $2_2^{LC}$ $3^B$ 4 | 1.7600 | 0.0405 | 1e-09 | 1e-07 | gauss |
| 1 $2_2^{LC}$ $3^B$ $4^B$ | 1.6689 | 0.0184 | 1e-09 | 1e-07 | gauss |
| 1 $2_3^{LC}$ | 1.6752 | 0.0399 | 1e-11 | 1e-07 | gauss |
| 1 $2_3^{LC}$ 3 | 1.6106 | 0.1316 | 1e-11 | 1e-07 | gauss |
| 1 $2_3^{LC}$ 3 4 | 1.7256 | 0.0412 | 1e-09 | 1e-07 | gauss |
| 1 $2_3^{LC}$ 3 4 5 | 1.8862 | 0.0808 | 1e-09 | 1e-07 | gauss |
| 1 $2_3^{LC}$ 3 $4^B$ | 1.4622 | 0.0437 | 1e-09 | 1e-07 | gauss |
| 1 $2_3^{LC}$ 3 $4^B$ 5 | 1.6017 | 0.0713 | 1e-09 | 1e-07 | gauss |
| 1 $2_3^{LC}$ $3^B$ | 1.4303 | 0.0317 | 1e-11 | 1e-07 | gauss |
| 1 $2_3^{LC}$ $3^B$ 4 | 1.5562 | 0.0576 | 1e-09 | 1e-07 | gauss |
| 1 $2_3^{LC}$ $3^B$ 4 5 | 1.7777 | 0.0792 | 1e-09 | 1e-07 | gauss |
| 1 $2_3^{LC}$ $3^B$ $4^B$ | 1.4481 | 0.0611 | 1e-09 | 1e-07 | gauss |
| 1 $2_3^{LC}$ $3^B$ $4^B$ 5 | 1.5975 | 0.0710 | 1e-09 | 1e-07 | gauss |
| 1 $2_3^{LC}$ {'$\beta$': 30.0} | 1.8162 | 0.0409 | 1e-07 | 1e-05 | gauss |
| 1 $2_3^{LC}$ {'$\beta$': 30.0} $3^B$ | 1.6015 | 0.0446 | 1e-07 | 1e-05 | gauss |
| 1 $2_3^{LC}$ {'$\beta$': 30.0} $3^B$ $4^B$ | 1.4172 | 0.0658 | 1e-09 | 1e-07 | gauss |

| | | | | | |
|---|---|---|---|---|---|
| 1 $2_3^{NC}$ | 1.8124 | 0.0431 | 1e-07 | 1e-05 | gauss |
| 1 $2_3^{NC}$ $3^B$ | 1.6005 | 0.0445 | 1e-07 | 1e-05 | gauss |
| 1 $2_3^{NC}$ $3^B$ $4^B$ | 1.4136 | 0.0648 | 1e-09 | 1e-07 | gauss |
| 1 $2_3^{NC}$ {'$\beta$': 30.0} | 1.7988 | 0.0466 | 1e-07 | 1e-05 | gauss |
| 1 $2_3^{NC}$ {'$\beta$': 30.0} $3^B$ | 1.5968 | 0.0430 | 1e-07 | 1e-05 | gauss |
| 1 $2_3^{NC}$ {'$\beta$': 30.0} $3^B$ $4^B$ | 1.4084 | 0.0595 | 1e-09 | 1e-07 | gauss |
| 1 $2_3^{NP}$ | 1.4487 | 0.0568 | 1e-09 | 1e-05 | gauss |
| 1 $2_3^{NP}$ $3^B$ | 1.1907 | 0.0413 | 1e-09 | 1e-05 | gauss |
| 1 $2_3^{NP}$ $3^B$ $4^B$ | 1.2534 | 0.0148 | 1e-07 | 1e-05 | gauss |
| 1 $2_3^{SC}$ | 2.5309 | 0.0563 | 1e-07 | 1e-07 | gauss |
| 1 $2_3^{SC}$ $3^B$ | 2.1568 | 0.0277 | 1e-07 | 1e-07 | gauss |
| 1 $2_3^{SC}$ $3^B$ $4^B$ | 1.7724 | 0.0485 | 1e-07 | 1e-07 | gauss |
| 1 $2_3^{SC}$ {'$\beta$': 30.0} | 2.5309 | 0.0563 | 1e-07 | 1e-07 | gauss |
| 1 $2_3^{SC}$ {'$\beta$': 30.0} $3^B$ | 2.1568 | 0.0277 | 1e-07 | 1e-07 | gauss |
| 1 $2_3^{SC}$ {'$\beta$': 30.0} $3^B$ $4^B$ | 1.7724 | 0.0485 | 1e-07 | 1e-07 | gauss |
| 1 $2_4^{LC}$ | 2.1115 | 0.0429 | 1e-09 | 1e-07 | gauss |
| 1 $2_4^{LC}$ 3 | 1.9871 | 0.0280 | 1e-09 | 1e-07 | gauss |
| 1 $2_4^{LC}$ 3 4 | 1.8957 | 0.0265 | 1e-09 | 1e-07 | gauss |
| 1 $2_4^{LC}$ 3 $4^B$ | 1.6755 | 0.0287 | 1e-09 | 1e-07 | gauss |
| 1 $2_4^{LC}$ $3^B$ | 1.7272 | 0.0316 | 1e-09 | 1e-07 | gauss |
| 1 $2_4^{LC}$ $3^B$ 4 | 1.6882 | 0.0395 | 1e-09 | 1e-07 | gauss |
| 1 $2_4^{LC}$ $3^B$ $4^B$ | 1.6408 | 0.0267 | 1e-09 | 1e-07 | gauss |
| 1 $2_5^{LC}$ | 2.1486 | 0.0434 | 1e-09 | 1e-07 | gauss |
| 1 $2_5^{LC}$ 3 | 2.0172 | 0.0360 | 1e-09 | 1e-07 | gauss |
| 1 $2_5^{LC}$ 3 4 | 1.9350 | 0.0256 | 1e-09 | 1e-07 | gauss |
| 1 $2_5^{LC}$ 3 $4^B$ | 1.7286 | 0.0320 | 1e-09 | 1e-07 | gauss |
| 1 $2_5^{LC}$ $3^B$ | 1.7978 | 0.0364 | 1e-09 | 1e-07 | gauss |

| | | | | | |
|---|---|---|---|---|---|
| 1 $2_5^{LC}$ $3^B$ 4 | 1.7653 | 0.0317 | 1e-09 | 1e-07 | gauss |
| 1 $2_5^{LC}$ $3^B$ $4^B$ | 1.7103 | 0.0262 | 1e-09 | 1e-07 | gauss |
| 1 $2_6^{LC}$ | 2.1624 | 0.0563 | 1e-09 | 1e-07 | gauss |
| 1 $2_6^{LC}$ 3 | 2.0330 | 0.0640 | 1e-09 | 1e-07 | gauss |
| 1 $2_6^{LC}$ 3 4 | 1.9336 | 0.0263 | 1e-09 | 1e-07 | gauss |
| 1 $2_6^{LC}$ 3 $4^B$ | 1.7354 | 0.0365 | 1e-09 | 1e-07 | gauss |
| 1 $2_6^{LC}$ $3^B$ | 1.8019 | 0.0335 | 1e-09 | 1e-07 | gauss |
| 1 $2_6^{LC}$ $3^B$ 4 | 1.7596 | 0.0307 | 1e-09 | 1e-07 | gauss |
| 1 $2_6^{LC}$ $3^B$ $4^B$ | 1.7146 | 0.0290 | 1e-09 | 1e-07 | gauss |
| 1 $2_7^{LC}$ | 2.1618 | 0.0593 | 1e-09 | 1e-07 | gauss |
| 1 $2_7^{LC}$ 3 | 2.0361 | 0.0683 | 1e-09 | 1e-07 | gauss |
| 1 $2_7^{LC}$ 3 4 | 1.9334 | 0.0288 | 1e-09 | 1e-07 | gauss |
| 1 $2_7^{LC}$ 3 $4^B$ | 1.7394 | 0.0387 | 1e-09 | 1e-07 | gauss |
| 1 $2_7^{LC}$ $3^B$ | 1.7999 | 0.0342 | 1e-09 | 1e-07 | gauss |
| 1 $2_7^{LC}$ $3^B$ 4 | 1.7602 | 0.0261 | 1e-09 | 1e-07 | gauss |
| 1 $2_7^{LC}$ $3^B$ $4^B$ | 1.7178 | 0.0330 | 1e-09 | 1e-07 | gauss |
| 1 Bag of Bonds | 2.6897 | 0.0420 | 1e-07 | 1e-07 | laplace |
| 1 Bag of Bonds 3 | 2.5241 | 0.0374 | 1e-07 | 1e-07 | laplace |
| 1 Bag of Bonds 3 4 | 2.4971 | 0.0219 | 1e-07 | 1e-07 | laplace |
| 1 Bag of Bonds 3 $4^B$ | 2.3190 | 0.0496 | 1e-07 | 1e-07 | laplace |
| 1 Bag of Bonds $3^B$ | 2.4431 | 0.0550 | 1e-07 | 1e-07 | laplace |
| 1 Bag of Bonds $3^B$ 4 | 2.4396 | 0.0386 | 1e-07 | 1e-07 | laplace |
| 1 Bag of Bonds $3^B$ $4^B$ | 2.3262 | 0.0461 | 1e-07 | 1e-07 | laplace |
| $1^C$ | 9.3266 | 0.1211 | 1e-07 | 1e-03 | gauss |
| $1^C$ $2^B$ | 6.6876 | 0.0054 | 1e-05 | 1e-03 | gauss |
| $1^C$ $2^B$ 3 | 5.0100 | 0.1493 | 1e-11 | 1e-07 | laplace |
| $1^C$ $2^B$ 3 4 | 3.4528 | 0.0977 | 1e-11 | 1e-07 | laplace |

| | | | | | |
|---|---|---|---|---|---|
| $1^C$ $2^B$ 3 4 5 | 3.7071 | 0.2631 | 1e-09 | 1e-07 | gauss |
| $1^C$ $2^B$ 3 $4^B$ | 4.1354 | 0.1190 | 1e-09 | 1e-07 | gauss |
| $1^C$ $2^B$ 3 $4^B$ 5 | 3.4048 | 0.1603 | 1e-07 | 1e-07 | gauss |
| $1^C$ $2^B$ $3^B$ | 4.4394 | 0.1219 | 1e-11 | 1e-07 | laplace |
| $1^C$ $2^B$ $3^B$ 4 | 3.3516 | 0.1076 | 1e-11 | 1e-07 | laplace |
| $1^C$ $2^B$ $3^B$ 4 5 | 3.3742 | 0.2473 | 1e-09 | 1e-07 | gauss |
| $1^C$ $2^B$ $3^B$ $4^B$ | 3.8367 | 0.1346 | 1e-11 | 1e-07 | laplace |
| $1^C$ $2^B$ $3^B$ $4^B$ 5 | 3.0883 | 0.1180 | 1e-09 | 1e-07 | gauss |
| $1^C$ ${}^{LC}2$ | 2.1566 | 0.0604 | 1e-09 | 1e-07 | gauss |
| $1^C$ $2^{LC}$ 3 | 2.0392 | 0.0682 | 1e-09 | 1e-07 | gauss |
| $1^C$ $2^{LC}$ 3 4 | 1.9410 | 0.0438 | 1e-09 | 1e-07 | gauss |
| $1^C$ $2^{LC}$ 3 $4^B$ | 1.7412 | 0.0440 | 1e-09 | 1e-07 | gauss |
| $1^C$ $2^{LC}$ $3^B$ | 1.8011 | 0.0456 | 1e-09 | 1e-07 | gauss |
| $1^C$ $2^{LC}$ $3^B$ 4 | 1.7589 | 0.0342 | 1e-09 | 1e-07 | gauss |
| $1^C$ $2^{LC}$ $3^B$ $4^B$ | 1.7131 | 0.0323 | 1e-09 | 1e-07 | gauss |
| $1^C$ $2_1^{LC}$ | 4.8068 | 0.0654 | 1e-07 | 1e-07 | laplace |
| $1^C$ $2_1^{LC}$ 3 | 4.2667 | 0.1048 | 1e-07 | 1e-07 | laplace |
| $1^C$ $2_1^{LC}$ 3 4 | 3.5751 | 0.0890 | 1e-09 | 1e-07 | gauss |
| $1^C$ $2_1^{LC}$ 3 $4^B$ | 3.1975 | 0.1186 | 1e-07 | 1e-07 | laplace |
| $1^C$ $2_1^{LC}$ $3^B$ | 3.8663 | 0.0792 | 1e-07 | 1e-07 | laplace |
| $1^C$ $2_1^{LC}$ $3^B$ 4 | 3.3696 | 0.1026 | 1e-09 | 1e-07 | gauss |
| $1^C$ $2_1^{LC}$ $3^B$ $4^B$ | 3.1662 | 0.0896 | 1e-07 | 1e-07 | laplace |
| $1^C$ $2_2^{LC}$ | 1.8295 | 0.0759 | 1e-11 | 1e-07 | gauss |
| $1^C$ $2_2^{LC}$ 3 | 1.8050 | 0.0523 | 1e-11 | 1e-07 | gauss |
| $1^C$ $2_2^{LC}$ 3 4 | 1.7256 | 0.0217 | 1e-11 | 1e-07 | gauss |
| $1^C$ $2_2^{LC}$ 3 $4^B$ | 1.6913 | 0.0144 | 1e-09 | 1e-07 | gauss |
| $1^C$ $2_2^{LC}$ $3^B$ | 1.7024 | 0.0744 | 1e-11 | 1e-07 | gauss |

| | | | | | |
|---|---|---|---|---|---|
| $1^C\ 2_2^{LC}\ 3^B\ 4$ | 1.7541 | 0.0452 | 1e-09 | 1e-07 | gauss |
| $1^C\ 2_2^{LC}\ 3^B\ 4^B$ | 1.6689 | 0.0180 | 1e-09 | 1e-07 | gauss |
| $1^C\ 2_3^{LC}$ | 1.6415 | 0.0531 | 1e-11 | 1e-07 | gauss |
| $1^C\ 2_3^{LC}\ 3$ | 1.5761 | 0.1235 | 1e-11 | 1e-07 | gauss |
| $1^C\ 2_3^{LC}\ 3\ 4$ | 1.5667 | 0.0710 | 1e-11 | 1e-07 | gauss |
| $1^C\ 2_3^{LC}\ 3\ 4^B$ | 1.4574 | 0.0500 | 1e-09 | 1e-07 | gauss |
| $1^C\ 2_3^{LC}\ 3^B$ | 1.4337 | 0.0448 | 1e-11 | 1e-07 | gauss |
| $1^C\ 2_3^{LC}\ 3^B\ 4$ | 1.5515 | 0.0631 | 1e-09 | 1e-07 | gauss |
| $1^C\ 2_3^{LC}\ 3^B\ 4^B$ | 1.4419 | 0.0565 | 1e-09 | 1e-07 | gauss |
| $1^C\ 2_3^{LC}\ 3\ 4\ 5$ | 1.8888 | 0.0783 | 1e-09 | 1e-07 | gauss |
| $1^C\ 2_3^{LC}\ 3\ 4^B\ 5$ | 1.6110 | 0.0648 | 1e-09 | 1e-07 | gauss |
| $1^C\ 2_3^{LC}\ 3^B\ 4\ 5$ | 1.7805 | 0.0736 | 1e-09 | 1e-07 | gauss |
| $1^C\ 2_3^{LC}\ 3^B\ 4^B\ 5$ | 1.5937 | 0.0615 | 1e-09 | 1e-07 | gauss |
| $1^C\ 2_4^{LC}$ | 2.0737 | 0.0453 | 1e-09 | 1e-07 | gauss |
| $1^C\ 2_4^{LC}\ 3$ | 1.9700 | 0.0327 | 1e-09 | 1e-07 | gauss |
| $1^C\ 2_4^{LC}\ 3\ 4$ | 1.8883 | 0.0328 | 1e-09 | 1e-07 | gauss |
| $1^C\ 2_4^{LC}\ 3\ 4^B$ | 1.6749 | 0.0275 | 1e-09 | 1e-07 | gauss |
| $1^C\ 2_4^{LC}\ 3^B$ | 1.7232 | 0.0256 | 1e-09 | 1e-07 | gauss |
| $1^C\ 2_4^{LC}\ 3^B\ 4$ | 1.6836 | 0.0331 | 1e-09 | 1e-07 | gauss |
| $1^C\ 2_4^{LC}\ 3^B\ 4^B$ | 1.6460 | 0.0305 | 1e-09 | 1e-07 | gauss |
| $1^C\ 2_5^{LC}$ | 2.1359 | 0.0449 | 1e-09 | 1e-07 | gauss |
| $1^C\ 2_5^{LC}\ 3$ | 2.0150 | 0.0563 | 1e-09 | 1e-07 | gauss |
| $1^C\ 2_5^{LC}\ 3\ 4$ | 1.9425 | 0.0515 | 1e-09 | 1e-07 | gauss |
| $1^C\ 2_5^{LC}\ 3\ 4^B$ | 1.7331 | 0.0420 | 1e-09 | 1e-07 | gauss |
| $1^C\ 2_5^{LC}\ 3^B$ | 1.7996 | 0.0420 | 1e-09 | 1e-07 | gauss |
| $1^C\ 2_5^{LC}\ 3^B\ 4$ | 1.7614 | 0.0382 | 1e-09 | 1e-07 | gauss |
| $1^C\ 2_5^{LC}\ 3^B\ 4^B$ | 1.7067 | 0.0304 | 1e-09 | 1e-07 | gauss |

| | | | | | |
|---|---|---|---|---|---|
| $1^C$ $2_6^{LC}$ | 2.1544 | 0.0569 | 1e-09 | 1e-07 | gauss |
| $1^C$ $2_6^{LC}$ 3 | 2.0354 | 0.0666 | 1e-09 | 1e-07 | gauss |
| $1^C$ $2_6^{LC}$ 3 4 | 1.9393 | 0.0469 | 1e-09 | 1e-07 | gauss |
| $1^C$ $2_6^{LC}$ 3 $4^B$ | 1.7394 | 0.0425 | 1e-09 | 1e-07 | gauss |
| $1^C$ $2_6^{LC}$ $3^B$ | 1.8042 | 0.0441 | 1e-09 | 1e-07 | gauss |
| $1^C$ $2_6^{LC}$ $3^B$ 4 | 1.7588 | 0.0383 | 1e-09 | 1e-07 | gauss |
| $1^C$ $2_6^{LC}$ $3^B$ $4^B$ | 1.7121 | 0.0284 | 1e-09 | 1e-07 | gauss |
| $1^C$ $2_7^{LC}$ | 2.1543 | 0.0618 | 1e-09 | 1e-07 | gauss |
| $1^C$ $2_7^{LC}$ 3 | 2.0381 | 0.0691 | 1e-09 | 1e-07 | gauss |
| $1^C$ $2_7^{LC}$ 3 4 | 1.9396 | 0.0432 | 1e-09 | 1e-07 | gauss |
| $1^C$ $2_7^{LC}$ 3 $4^B$ | 1.7434 | 0.0431 | 1e-09 | 1e-07 | gauss |
| $1^C$ $2_7^{LC}$ $3^B$ | 1.8012 | 0.0454 | 1e-09 | 1e-07 | gauss |
| $1^C$ $2_7^{LC}$ $3^B$ 4 | 1.7592 | 0.0334 | 1e-09 | 1e-07 | gauss |
| $1^C$ $2_7^{LC}$ $3^B$ $4^B$ | 1.7154 | 0.0312 | 1e-09 | 1e-07 | gauss |
| $1^C$ Bag of Bonds | 2.6704 | 0.0481 | 1e-07 | 1e-07 | laplace |
| $1^C$ Bag of Bonds 3 | 2.5023 | 0.0458 | 1e-07 | 1e-07 | laplace |
| $1^C$ Bag of Bonds 3 4 | 2.4678 | 0.0267 | 1e-07 | 1e-07 | laplace |
| $1^C$ Bag of Bonds 3 $4^B$ | 2.3144 | 0.0553 | 1e-07 | 1e-07 | laplace |
| $1^C$ Bag of Bonds $3^B$ | 2.4218 | 0.0532 | 1e-07 | 1e-07 | laplace |
| $1^C$ Bag of Bonds $3^B$ 4 | 2.4156 | 0.0376 | 1e-07 | 1e-07 | laplace |
| $1^C$ Bag of Bonds $3^B$ $4^B$ | 2.3197 | 0.0511 | 1e-07 | 1e-07 | laplace |
| 2 | 27.0143 | 1.2266 | 1e-11 | 1e-05 | gauss |
| $2^B$ | 7.6924 | 0.1527 | 1e-07 | 1e-03 | gauss |
| $2^{LP}$ | 3.1836 | 0.1023 | 1e-09 | 1e-05 | gauss |
| $2^{NC}$ | 2.9543 | 0.0646 | 1e-09 | 1e-07 | gauss |
| $2^{NP}$ | 3.4914 | 0.1005 | 1e-07 | 1e-05 | gauss |
| $2^{NP}$ {'end': 12.0} | 4.0497 | 0.0908 | 1e-09 | 1e-05 | gauss |

| | | | | | |
|---|---|---|---|---|---|
| $2^{NP}$ {'end': 16.0} | 8.8295 | 0.1648 | 1e-09 | 1e-05 | gauss |
| $2^{NP}$ {'end': 2.0} | 3.9053 | 0.5433 | 1e-09 | 1e-05 | gauss |
| $2^{NP}$ {'end': 4.0} | 2.8394 | 0.1226 | 1e-09 | 1e-05 | gauss |
| $2^{NP}$ {'end': 6.0} | 3.4914 | 0.1005 | 1e-07 | 1e-05 | gauss |
| $2^{NP}$ {'end': 8.0} | 3.5837 | 0.0939 | 1e-07 | 1e-05 | gauss |
| $2^{NP}$ {'segments': 10} | 51.6721 | 0.8192 | 1e-09 | 1e-05 | gauss |
| $2^{NP}$ {'segments': 150} | 3.3189 | 0.0993 | 1e-07 | 1e-05 | gauss |
| $2^{NP}$ {'segments': 200} | 3.2660 | 0.1039 | 1e-07 | 1e-05 | gauss |
| $2^{NP}$ {'segments': 25} | 21.2022 | 0.3948 | 1e-09 | 1e-05 | gauss |
| $2^{NP}$ {'segments': 50} | 3.8189 | 0.1564 | 1e-09 | 1e-05 | gauss |
| $2^{NP}$ {'segments': 75} | 3.3082 | 0.0701 | 1e-09 | 1e-05 | gauss |
| $2^{NP}$ {'$\beta$': 1.0} | 3.8716 | 0.1001 | 1e-07 | 1e-05 | gauss |
| $2^{NP}$ {'$\beta$': 10.0} | 3.1849 | 0.0777 | 1e-07 | 1e-05 | gauss |
| $2^{NP}$ {'$\beta$': 2.5} | 3.0443 | 0.1656 | 1e-09 | 1e-05 | gauss |
| $2^{NP}$ {'$\beta$': 30.0} | 3.5714 | 0.1258 | 1e-09 | 1e-05 | gauss |
| $2^{NP}$ {'$\beta$': 40.0} | 4.4723 | 0.1251 | 1e-09 | 1e-05 | gauss |
| $2^{NP}$ {'$\beta$': 5.0} | 3.1355 | 0.0516 | 1e-07 | 1e-05 | gauss |
| $2^{NP}$ {'$\beta$': 80.0} | 35.0504 | 0.8029 | 1e-07 | 1e-05 | gauss |
| $2^{NP}$ {'start': 0.1} | 3.4565 | 0.0847 | 1e-07 | 1e-05 | gauss |
| $2^{NP}$ {'start': 0.2} | 3.4914 | 0.1005 | 1e-07 | 1e-05 | gauss |
| $2^{NP}$ {'start': 0.4} | 3.4549 | 0.1007 | 1e-07 | 1e-05 | gauss |
| $2^{NP}$ {'start': 0.8} | 3.4270 | 0.0983 | 1e-07 | 1e-05 | gauss |
| $2^{NP}$ {'start': 1.0} | 3.4181 | 0.0877 | 1e-07 | 1e-05 | gauss |
| $2^{NP}$ {'start': 1.5} | 7.2008 | 0.0602 | 1e-07 | 1e-05 | gauss |
| $2^{SC}$ | 4.0910 | 0.0993 | 1e-07 | 1e-07 | gauss |
| $2^{SP}$ | 132.0560 | 3.0004 | 1e-09 | 1e-11 | gauss |
| $2_1$ | 6.3495 | 0.1191 | 1e-07 | 1e-07 | laplace |

| | | | | | |
|---|---|---|---|---|---|
| $2_1^{LP}$ | 7.5691 | 1.6200 | 1e-09 | 1e-05 | gauss |
| $2_1^{NC}$ | 6.4204 | 0.6765 | 1e-07 | 1e-05 | gauss |
| $2_1^{NP}$ | 6.2499 | 2.0349 | 1e-11 | 1e-05 | gauss |
| $2_1^{SC}$ | 6.2928 | 0.1868 | 1e-09 | 1e-05 | gauss |
| $2_1^{SP}$ | 167.2493 | 1.5730 | 1e-09 | 1e-05 | gauss |
| $2_2$ | 3.3990 | 0.5837 | 1e-11 | 1e-07 | gauss |
| $2_2^{LP}$ | 2.5101 | 0.1446 | 1e-11 | 1e-05 | gauss |
| $2_2^{NC}$ | 2.7340 | 0.0770 | 1e-07 | 1e-05 | gauss |
| $2_2^{NP}$ | 2.4360 | 0.3073 | 1e-11 | 1e-05 | gauss |
| $2_2^{SC}$ | 3.1870 | 0.0630 | 1e-07 | 1e-05 | gauss |
| $2_2^{SP}$ | 160.7898 | 1.6727 | 1e-07 | 1e-05 | gauss |
| $2_3$ | 2.7405 | 0.0779 | 1e-11 | 1e-07 | gauss |
| $2_3^{LC}$ | 2.7402 | 0.0769 | 1e-11 | 1e-07 | gauss |
| $2_3^{LC}$ {'$\beta$': 30.0} | 2.7213 | 0.0613 | 1e-11 | 1e-07 | gauss |
| $2_3^{LP}$ | 2.6063 | 0.0714 | 1e-09 | 1e-05 | gauss |
| $2_3^{NC}$ | 2.7179 | 0.0776 | 1e-11 | 1e-07 | gauss |
| $2_3^{NC}$ $2_3^{NP}$ | 2.8589 | 0.0621 | 1e-09 | 1e-07 | gauss |
| $2_3^{NC}$ {'$\beta$': 30.0} | 2.8776 | 0.0932 | 1e-09 | 1e-07 | gauss |
| $2_3^{NP}$ | 2.4520 | 0.0817 | 1e-09 | 1e-05 | gauss |
| $2_3^{NP}$ {'end': 12.0} | 3.3002 | 0.0953 | 1e-09 | 1e-05 | gauss |
| $2_3^{NP}$ {'end': 16.0} | 8.4140 | 0.2894 | 1e-09 | 1e-05 | gauss |
| $2_3^{NP}$ {'end': 4.0} | 2.3865 | 0.0690 | 1e-09 | 1e-05 | gauss |
| $2_3^{NP}$ {'end': 6.0} | 2.4520 | 0.0817 | 1e-09 | 1e-05 | gauss |
| $2_3^{NP}$ {'end': 8.0} | 2.5219 | 0.0522 | 1e-09 | 1e-05 | gauss |
| $2_3^{NP}$ {'segments': 10} | 76.5502 | 1.1925 | 1e-09 | 1e-05 | gauss |
| $2_3^{NP}$ {'segments': 150} | 2.3723 | 0.0879 | 1e-09 | 1e-05 | gauss |
| $2_3^{NP}$ {'segments': 200} | 2.3724 | 0.0866 | 1e-09 | 1e-05 | gauss |

| | | | | | |
|---|---|---|---|---|---|
| $2_3^{NP}$ {'segments': 25} | 22.3027 | 0.3675 | 1e-09 | 1e-05 | gauss |
| $2_3^{NP}$ {'segments': 50} | 3.3063 | 0.1420 | 1e-09 | 1e-05 | gauss |
| $2_3^{NP}$ {'segments': 75} | 2.5052 | 0.0509 | 1e-09 | 1e-05 | gauss |
| $2_3^{NP}$ {'$\beta$': 1.0} | 6.2651 | 0.0677 | 1e-09 | 1e-05 | gauss |
| $2_3^{NP}$ {'$\beta$': 10.0} | 2.4681 | 0.0623 | 1e-09 | 1e-05 | gauss |
| $2_3^{NP}$ {'$\beta$': 2.5} | 3.8039 | 0.0425 | 1e-09 | 1e-05 | gauss |
| $2_3^{NP}$ {'$\beta$': 30.0} | 2.5371 | 0.1042 | 1e-09 | 1e-05 | gauss |
| $2_3^{NP}$ {'$\beta$': 40.0} | 3.5383 | 0.1359 | 1e-09 | 1e-05 | gauss |
| $2_3^{NP}$ {'$\beta$': 5.0} | 3.0443 | 0.1656 | 1e-09 | 1e-05 | gauss |
| $2_3^{NP}$ {'$\beta$': 80.0} | 37.2210 | 1.4209 | 1e-09 | 1e-05 | gauss |
| $2_3^{NP}$ {'start': 0.1} | 2.4346 | 0.0895 | 1e-09 | 1e-05 | gauss |
| $2_3^{NP}$ {'start': 0.2} | 2.4520 | 0.0817 | 1e-09 | 1e-05 | gauss |
| $2_3^{NP}$ {'start': 0.4} | 2.4326 | 0.0919 | 1e-09 | 1e-05 | gauss |
| $2_3^{NP}$ {'start': 0.8} | 2.3938 | 0.0946 | 1e-09 | 1e-05 | gauss |
| $2_3^{NP}$ {'start': 1.0} | 2.4019 | 0.0934 | 1e-09 | 1e-05 | gauss |
| $2_3^{NP}$ {'start': 1.5} | 10.8269 | 0.2624 | 1e-09 | 1e-05 | gauss |
| $2_3^{SC}$ | 3.6489 | 0.1096 | 1e-09 | 1e-07 | gauss |
| $2_3^{SC}$ {'$\beta$': 30.0} | 3.6489 | 0.1096 | 1e-09 | 1e-07 | gauss |
| $2_3^{SP}$ | 146.4782 | 2.6895 | 1e-07 | 1e-05 | gauss |
| $2_4$ | 3.3554 | 0.0558 | 1e-09 | 1e-07 | gauss |
| $2_4^{LP}$ | 2.9515 | 0.1458 | 1e-09 | 1e-05 | gauss |
| $2_4^{NC}$ | 3.1824 | 0.0796 | 1e-09 | 1e-07 | gauss |
| $2_4^{NP}$ | 3.0073 | 0.1094 | 1e-09 | 1e-05 | gauss |
| $2_4^{SC}$ | 4.1667 | 0.0960 | 1e-09 | 1e-07 | gauss |
| $2_4^{SP}$ | 141.7759 | 3.3160 | 1e-05 | 1e-07 | gauss |
| $2_5$ | 3.5451 | 0.0708 | 1e-09 | 1e-07 | gauss |
| $2_5^{LP}$ | 3.3860 | 0.1120 | 1e-09 | 1e-05 | gauss |

| | | | | | |
|---|---|---|---|---|---|
| $2_5^{NC}$ | 3.4412 | 0.0751 | 1e-09 | 1e-07 | gauss |
| $2_5^{NP}$ | 3.4864 | 0.0987 | 1e-09 | 1e-05 | gauss |
| $2_5^{SC}$ | 4.5364 | 0.0881 | 1e-09 | 1e-07 | gauss |
| $2_5^{SP}$ | 136.2433 | 3.4077 | 1e-09 | 1e-11 | gauss |
| $2_6$ | 3.5102 | 0.0700 | 1e-09 | 1e-07 | gauss |
| $2_6^{LP}$ | 3.4702 | 0.1062 | 1e-09 | 1e-05 | gauss |
| $2_6^{NC}$ | 3.3962 | 0.0546 | 1e-09 | 1e-07 | gauss |
| $2_6^{NP}$ | 3.7576 | 0.0970 | 1e-07 | 1e-05 | gauss |
| $2_6^{SC}$ | 4.5080 | 0.0667 | 1e-09 | 1e-07 | gauss |
| $2_6^{SP}$ | 133.9029 | 2.8934 | 1e-09 | 1e-11 | gauss |
| $2_7$ | 3.5038 | 0.0731 | 1e-09 | 1e-07 | gauss |
| $2_7^{LP}$ | 3.4846 | 0.1020 | 1e-09 | 1e-05 | gauss |
| $2_7^{NC}$ | 3.3877 | 0.0630 | 1e-09 | 1e-07 | gauss |
| $2_7^{NP}$ | 3.7627 | 0.0946 | 1e-07 | 1e-05 | gauss |
| $2_7^{SC}$ | 4.4929 | 0.0669 | 1e-09 | 1e-07 | gauss |
| $2_7^{SP}$ | 133.4427 | 2.8907 | 1e-09 | 1e-11 | gauss |
| 3 | 45.2756 | 1.5846 | 1e-05 | 1e-03 | gauss |
| $3^B$ | 6.3598 | 0.2685 | 1e-11 | 1e-07 | gauss |
| 4 | 64.2473 | 1.0873 | 1e-11 | 1e-07 | laplace |
| $4^B$ | 51.4362 | 1.2445 | 1e-11 | 1e-07 | laplace |
| 5 | 56.4299 | 3.4445 | 1e-03 | 1e-03 | laplace |
| $5^B$ | 67.4268 | 2.0270 | 1e-05 | 1e-05 | gauss |
| Bag of Bonds | 2.4137 | 0.0302 | 1e-09 | 1e-03 | laplace |
| Bag of Bonds {'strip atoms': True} | 2.3973 | 0.0353 | 1e-09 | 1e-03 | laplace |
| Bag of $\text{Bonds}_1$ | 3.3332 | 0.0958 | 1e-05 | 1e-03 | laplace |
| Bag of $\text{Bonds}_1$ {'strip atoms': True} | 3.7842 | 0.1366 | 1e-05 | 1e-03 | laplace |
| Bag of $\text{Bonds}_2$ | 2.1441 | 0.0892 | 1e-07 | 1e-05 | laplace |

| | | | | | |
|---|---|---|---|---|---|
| Bag of Bonds$_2$ {'strip atoms': True} | 3.1378 | 0.0975 | 1e-09 | 1e-03 | laplace |
| Bag of Bonds$_3$ | 2.3332 | 0.0880 | 1e-07 | 1e-05 | laplace |
| Bag of Bonds$_3$ {'strip atoms': True} | 3.7245 | 0.1495 | 1e-09 | 1e-05 | laplace |
| Bag of Bonds$_4$ | 2.5566 | 0.0916 | 1e-07 | 1e-05 | laplace |
| Bag of Bonds$_4$ {'strip atoms': True} | 3.8601 | 0.0667 | 1e-09 | 1e-03 | laplace |
| Bag of Bonds$_5$ | 2.6012 | 0.1162 | 1e-07 | 1e-05 | laplace |
| Bag of Bonds$_5$ {'strip atoms': True} | 3.8341 | 0.0725 | 1e-09 | 1e-03 | laplace |
| Bag of Bonds$_6$ | 2.5947 | 0.0917 | 1e-07 | 1e-05 | laplace |
| Bag of Bonds$_6$ {'strip atoms': True} | 3.8087 | 0.0873 | 1e-09 | 1e-03 | laplace |
| Bag of Bonds$_7$ | 2.5660 | 0.0843 | 1e-07 | 1e-05 | laplace |
| Bag of Bonds$_7$ {'strip atoms': True} | 3.7550 | 0.0936 | 1e-09 | 1e-03 | laplace |
| Coulomb Matrix | 3.3714 | 0.1643 | 1e-07 | 1e-03 | laplace |
| Coulomb Matrix$_1$ | 2.8048 | 0.1232 | 1e-07 | 1e-03 | laplace |
| Coulomb Matrix$_2$ | 2.9136 | 0.1867 | 1e-07 | 1e-03 | laplace |
| Coulomb Matrix$_3$ | 3.2354 | 0.1384 | 1e-07 | 1e-03 | laplace |
| Coulomb Matrix$_4$ | 3.4033 | 0.1562 | 1e-07 | 1e-03 | laplace |
| Coulomb Matrix$_5$ | 3.3810 | 0.1651 | 1e-07 | 1e-03 | laplace |
| Coulomb Matrix$_6$ | 3.3332 | 0.1533 | 1e-07 | 1e-03 | laplace |
| Coulomb Matrix$_7$ | 3.3273 | 0.1582 | 1e-07 | 1e-03 | laplace |
| Null | 179.0135 | 0.0754 | 1e-09 | 1e-11 | gauss |

Table S4: KRR Results
